# Supplementary material for: ANISE: Assembly-based Neural Implicit Surface rEconstruction
Source: arXiv:2205.13682 source file (2023-07-05)
Supplement: Supplementary file 4 [file end_to_end_comparison.tex]

\begin{table}
\centering
%\resizebox{\linewidth}{!}{ %< auto-adjusts font size to fill line
\begin{tabular}{@{}lccc}
\toprule
Method & IoU ($\uparrow$) & CD ($\downarrow$) & F1 ($\uparrow$)  \\
\midrule
%PQ-Net 256 && - & 2.86 & - & 4.50\\
Ours (scratch) & 64.3 &   2.08 & 69.8 \\
%Ours-RFULL & 49.6 & 3.37 &  35.7 & 46.0 & 4.94 & 43.9\\ 
Ours (multi-stage) & 68.6 & 1.58 & 74.2  \\ 
\bottomrule
\end{tabular}
%} % \resizebox
\caption{
\textbf{Two stage training vs. end-to-end training.} Our multi-stage training described in Section \ref{sec:training} performs much better compared to training from scratch according to all measures. Comparison was done on the Chair category.
%with $M = 20$ parts.
% 
} % \caption
\label{tab:end_to_end_comparison}
\end{table}
